# Supplementary material for: Comparative structural evolution under pressure of powder and single crystals of the layered antiferromagnet FePS$_3$
Source: arXiv:2203.07015 ancillary file (2022-03-14)
Supplement: Supplementary file 1 [file SupplementaryText.pdf]

## **Supplementary information for Comparative structural evolution under pressure of powder and single crystals of the layered antiferromagnet FePS<sub>3</sub>**

D. M. Jarvis, M. J. Coak, H. Hamidov, C. R. S. Haines, G. I. Lampronti, C. Liu, S. Deng, D. Daisenberger, D. R. Allan, M. R. Warren, A. R. Wildes, S. S. Saxena

### ***Proposed models from existing literature***

Various complementary methods were used to select the correct structure for the HP-II phase of FePS<sub>3</sub> from between the models proposed in literature: that of Haines et al.<sup>1</sup>, with the HP-I to HP-II transition involving an increase in symmetry from space group C2/m to P-31m and a collapse of the inter-planar spacing of ~15%; and that proposed by Wang et al.<sup>2</sup> which maintains a monoclinic symmetry and proposes a volume collapse arising instead from a simultaneous reduction in the intra-planar lattice parameters.

### ***Determination of distances from reciprocal space images***

To examine the correctness of the single-crystal unit cell refinements performed on Crysalis Pro<sup>3</sup>, slices through different planes of reciprocal space were taken using the software and the visible spots examined directly to determine characteristic distances of the unit cell.

Figure S1 shows simulated diffraction patterns of FePS<sub>3</sub> for the plane normal to the  $c^*$  axis in the three distinct structural phases along with the corresponding observed patterns from the single-crystal diffraction data. The transition to the HP-I phase is most clearly demonstrated by the observation of the hexagon of spots visible inside the innermost powder rings that arise from the rhenium gasket, indexed as the  $(\pm 2\ 0\ 0)$  and  $(\pm 1\ \pm 3\ 0)$  peaks, which are absent in the ambient-pressure phase. The transition from the HP-I to HP-II phase is more pronounced in the observations of inter-planar spacing noted in the main text and shown in reciprocal space images by changes of spot position along directions parallel to  $c^*$  as in Figure 1 of the main text.

For determination of both the inter-planar spacing and a characteristic Fe-Fe distance within the honeycombs, planes containing the three pairs of spots forming the characteristic hexagon containing the monoclinic  $(0\ 6\ 0)$  or trigonal  $(0\ 3\ 0)$  spots in Figure S1 were examined.

This selection of slices is justified by the presence of rotational twins in the material differing by a rotation of 120° around the vector normal to the  $ab$  planes, being the real space  $[103]$  direction in the HP-0 phase<sup>4</sup> and  $[001]$  in the HP-I and HP-II phases where  $\beta \approx 90^\circ$ . When rotated by 120°, the  $(0\ k\ 0)$  spots overlap others arising from the original twin which are indexed as shown in Figure S1. Bitmaps of reciprocal space images as in Figure 1 of the main text were generated, where the vertical direction is  $(0\ 0\ l)$  and the horizontal direction was either  $(0\ k\ 0)$ ,  $(3h\ 3h\ -l)$  or  $(-3h\ 3h\ l)$  for HP-0;  $(0\ k\ 0)$ ,  $(3h\ 3h\ 0)$  or  $(-3h\ 3h\ 0)$  for HP-I;  $(0\ k\ 0)$ ,  $(h\ 0\ 0)$  or  $(-3h\ 3h\ 0)$  for HP-II in order to capture the spots of interest.

From these images, the resolution of  $Q$  in  $\text{\AA}^{-1}/\text{pixel}$  of the output images was determined from the Crysalis Pro settings and verified by the overlaid reciprocal lattice grid output by the software. A window wide enough to capture the diffraction spots of interest, typically 5 pixels, was taken and integrated along the horizontal direction, giving a one-dimensional dataset of integrated intensity as a function of  $Q$  in  $\text{\AA}^{-1}$  along  $(0\ 0\ l)$ . An example slice and the resultant integrated intensity is shown in Figure S2. To these data, gaussian peaks plus a background were fit to the peaks of interest, e.g.  $(0\ 6\ 0)$  and  $(0\ 6\ \pm 1)$ , and the distance in reciprocal space between these peaks determined from these fits. This then is simply converted to a real space distance representing the inter-planar distance.

Similarly, the  $Q$  distance along the horizontal direction of the images between the monoclinic  $(0\ 6\ 0)$  and  $(0\ -6\ 0)$  or rotationally equivalent peaks is determined through integrating vertically a narrow band encompassing the spots. The  $(0\ 6\ 0)$  spacing is determined from this, which is approximately half of the Fe-Fe distance in the honeycomb (see the inset of Figure 3 in the main text). This characteristic intra-planar distance is determined on the assumption of perfect hexagons in the  $ab$  planes, deviations from which in the monoclinic phases are very small.

The use of three pairs of  $l=0$  peaks and those adjacent along  $l$  allows for a useful redundancy for these calculations. From each pressure set of slices, for the inter-planar spacing (being the real space distance between  $(0\ 0\ 1)$  planes), at most twelve values may be taken; and for the intra-planar value, three values are always found. In many cases, fewer than twelve measurements are possible for the inter-planar spacing due to either the positive or negative  $l$  peak being outside the window of reciprocal space accessible from the geometry of the pressure cell.

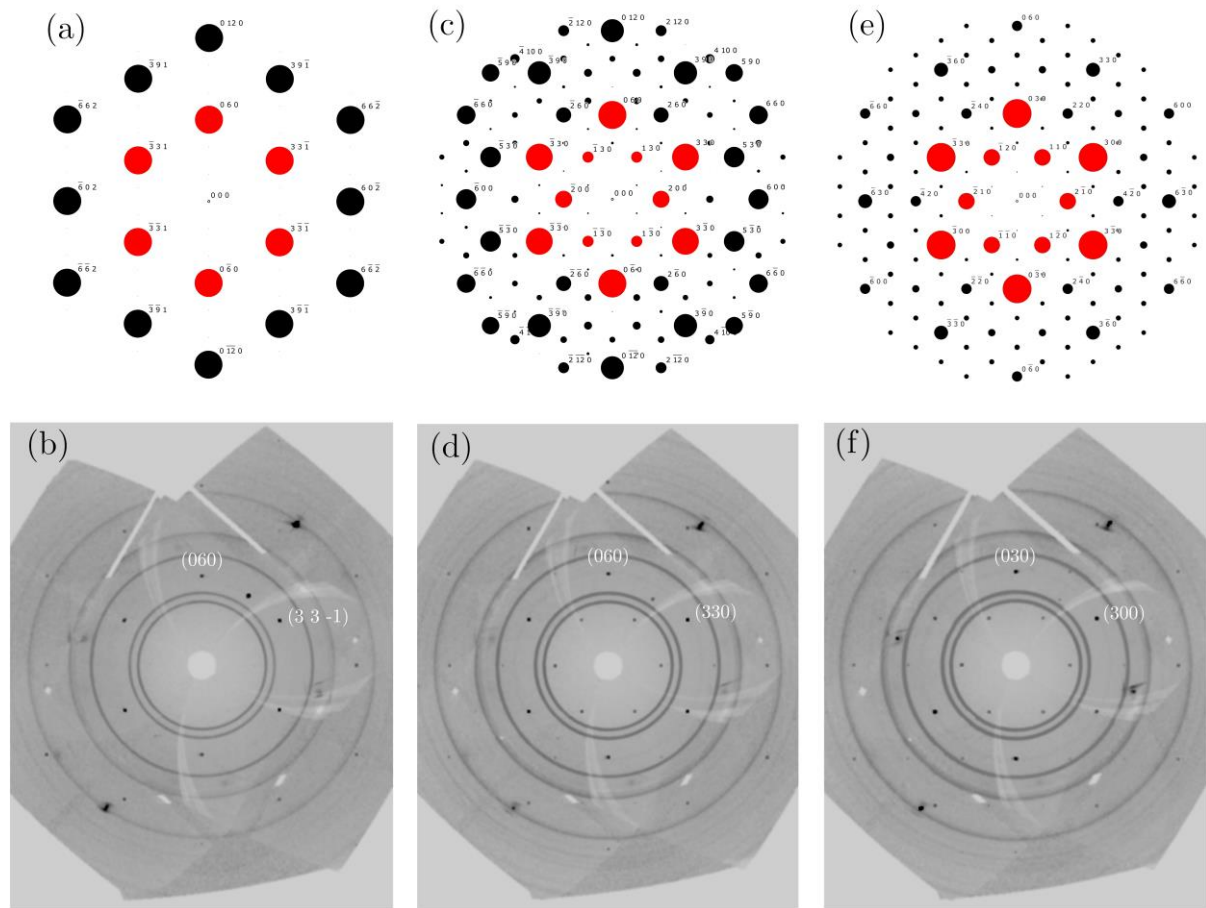

**Figure S1** – Simulated and experimentally observed reciprocal space images for (a, b) the HP-0 monoclinic phase at 1 GPa; (c, d) the HP-I monoclinic phase at 10 GPa; (e, f) the HP-II trigonal phase at 19 GPa. The clearest peaks in the observed data are highlighted red in the simulations. The  $c^*$  direction is normal to the page.

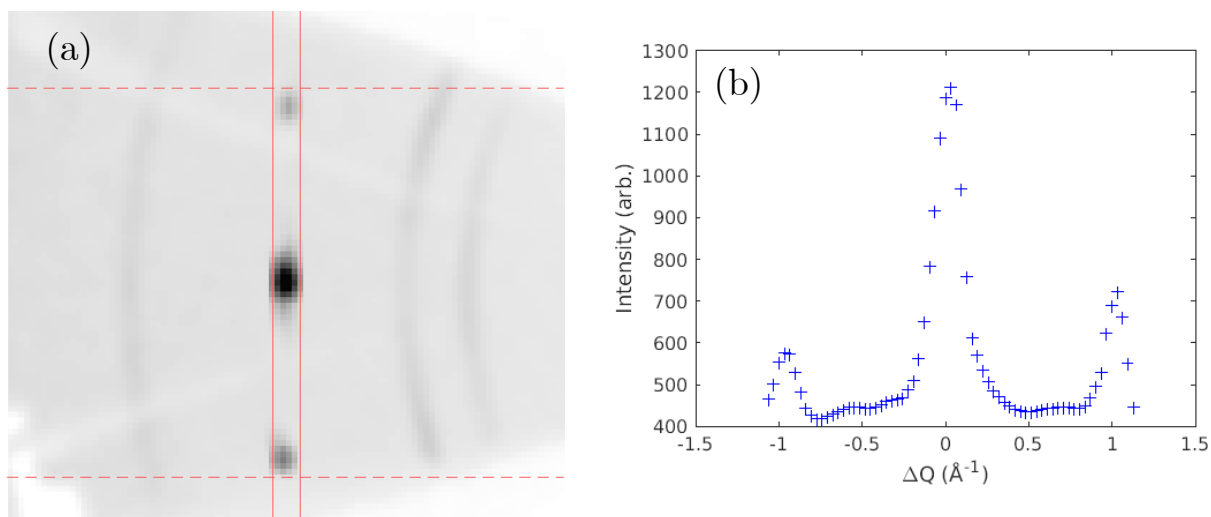

**Figure S2** – (a) Section of the  $(0\ k\ l)$  scattering plane showing the  $(0\ -6\ -1)$ ,  $(0\ -6\ 0)$  and  $(0\ -6\ 1)$  spots of  $\text{FePS}_3$  at 0.4 GPa and the window in red over which intensity was integrated horizontally with dashed lines showing the vertical limits; (b) the resultant plot of integrated intensity along the vertical  $(0\ -6\ l)$  direction, where the horizontal axis is distance in reciprocal space from the centre of the slice.

### Single crystal unit cell refinement using CrysAlis Pro

Unit cells for the three structural phases of  $\text{FePS}_3$  determined from the single-crystal diffraction experiment are given in Table S1. These were found through standard procedure within the software, with initial cells determined from peak searches then constrained according to the determined space group.

|                           |                           |                          |                             |
|---------------------------|---------------------------|--------------------------|-----------------------------|
| <b>HP-0</b> – 1.2 GPa     | C2/m                      | Comp. = 37.99%           | $R_{\text{int}} = 0.1256$   |
| <b>a (Å)</b><br>5.804(12) | <b>b (Å)</b><br>10.030(6) | <b>c (Å)</b><br>7.08(10) | <b>β (deg)</b><br>106.9(7)  |
| <b>HP-I</b> – 6.7 GPa     | C2/m                      | Comp. = 26.97%           | $R_{\text{int}} = 0.0880$   |
| <b>a (Å)</b><br>5.802(2)  | <b>b (Å)</b><br>10.056(4) | <b>c (Å)</b><br>5.95(7)  | <b>β (deg)</b><br>89.95(13) |
| <b>HP-II</b> – 20.1 GPa   | P-31m                     | Comp. = 30.83%           | $R_{\text{int}} = 0.2056$   |
| <b>a (Å)</b><br>5.665(4)  | <b>c (Å)</b><br>5.02(9)   |                          |                             |

**Table S1** – Lattice parameters, space groups, completeness and  $R_{\text{int}}$  for the three phases as determined from single crystal data using CrysAlis Pro.

## Coexistence of phases

Figures S3 and S4 show ranges of powder diffraction measurements of  $\text{FePS}_3$  at increasing pressure without a pressure medium, and Figure S5 a range from measurements taken with a helium medium. The no media data show clear coexistence of peaks across a range of  $\sim 3$  GPa around the HP-I to HP-II transition, which is not apparent for the data measured with a He medium. Similar phase coexistence is seen in the no medium data for the HP-0 to HP-I transition. The coexistence of phases is not observed in the measurements of single crystal  $\text{FePS}_3$ : at no point are peaks attributed to multiple structures observed simultaneously.

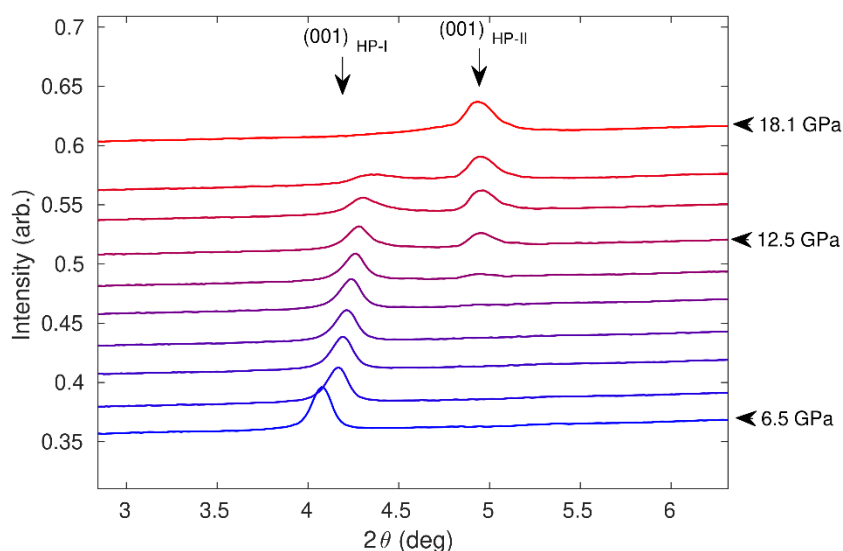

**Figure S3** – Powder diffraction patterns of  $\text{FePS}_3$  as a function of pressure measured without a pressure medium, showing the evolution of the (001) peak across the HP-I to HP-II transition. The simultaneous observation of the two phases is seen around the transition at 14 GPa.

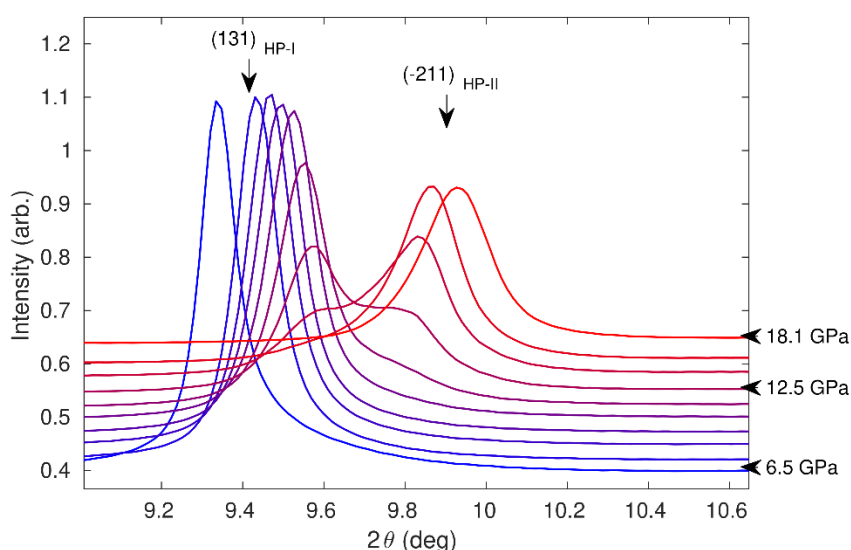

**Figure S4** – Powder diffraction patterns of  $\text{FePS}_3$  as a function of pressure measured without a pressure medium, showing the evolution of the monoclinic (131) peak to the trigonal (-2,1,1) across the HP-I to HP-II transition. The simultaneous observation of the two phases is seen around the transition at 14 GPa.

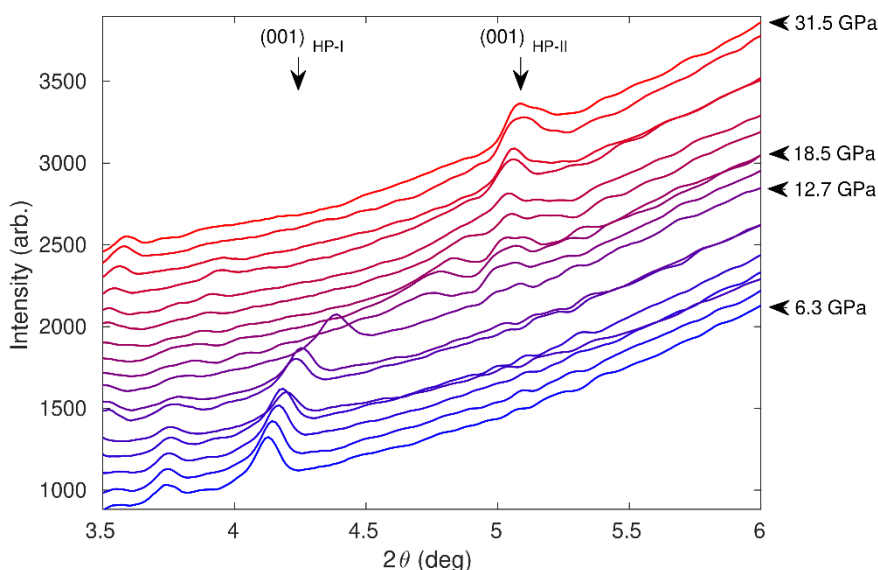

**Figure S5** – Powder diffraction measurements of FePS<sub>3</sub> as a function of pressure measured with a helium pressure medium, showing the evolution of the (001) peak across the HP-I to HP-II transition.

### ***Details of powder diffraction data analysis methods***

Rietveld refinements were performed with software Topas Academic V6.<sup>5</sup> The parameters describing the diffraction geometry and Pseudo-Voigt function used to model the peak shape were first optimized using an LaB<sub>6</sub> standard. These were fixed for the structural refinements. We here remind that the estimated standard deviation (e.s.d.) from the Rietveld calculation has no bearing on the precision or accuracy, but is merely related to the mathematical fit of the model.<sup>6</sup> So long as the same approach is used for all scans within a dataset, trends are reliable. While the visual inspection of a Rietveld plot is the most reliable way to determine the quality of a fit, this is not practical for larger datasets. A global check of a sequential refinement can be efficiently performed by comparing a number of “goodness of fit” indices,  $R_{wp}$  and  $\chi^2$ .<sup>7</sup>

### **DETERMINATION OF THE CORRECT STRUCTURE FOR THE HP-II PHASE**

#### ***Rietveld refinement of the HP-II models for powders in a He medium at 18.5 GPa, and with no media at 18.1 GPa.***

A shifted Chebyshev function with 6 parameters was used to fit the background. Structural parameters were refined with an anti-bump restraint for the P-P interatomic distance. Minimum and maximum values of 0.1 Å<sup>2</sup> and 1 Å<sup>2</sup> were set for the thermal parameters (one for each atomic species). Spherical harmonics were used to model preferred orientation. Two isotropic Lorentzian parameters were used to model the sample contribution to peak broadening for crystal size and microstrain respectively. The refinement for HP-II using Haines et al.’s model in He medium at 18.5 GPa converged with  $R_{wp}$  and  $\chi^2$  equal to 0.55% and 0.68 respectively. The Rietveld refinement plot is shown in Figure S6. The input file (223613\_He\_HP2\_P-31m\_18p5GPa\_Rietveld.inp), integrated data (223613.xy), and cif file (223613\_He\_HP2\_P-31m\_18p5GPa\_Rietveld.cif) for the so refined structure are included in the provided supplementary information. The refinement for HP-II using Wang et al.’s model in He medium at 18.5 GPa converged with  $R_{wp}$  and  $\chi^2$  equal to 0.54% and 0.68 respectively. The Rietveld refinement plot is shown in Figure S7. The input file

(223613\_He\_HP2\_C2\_m\_18p5GPa\_Rietveld.inp), integrated data (223613.xy), and cif file (223613\_He\_HP2\_C2\_m\_18p5GPa\_Rietveld.cif) for the so refined structure are included in the provided supplementary information. The refinement for HP-II (Haines et al.'s model) with no media at 18.1 GPa converged with  $R_{wp}$  and  $\chi^2$  equal to 0.55% and 0.68 respectively. The Rietveld refinement plot is shown in Figure S8. The input file (223663\_nomedia\_HP2\_P-31m\_18p1GPa\_Rietveld.inp), integrated data (223663.xy), and cif file (223663\_nomedia\_HP2\_P-31m\_18p1GPa\_Rietveld.cif) for the so refined structure are included in the provided supplementary information. The refinement for HP-II using Wang et al.'s model with no pressure medium at 18.1 GPa converged with  $R_{wp}$  and  $\chi^2$  equal to 2.63% and 1.22 respectively. The Rietveld refinement plot is shown in Figure S9. The input file (223663\_He\_HP2\_C2\_m\_18p1GPa\_Rietveld.inp), integrated data (223663.xy), and cif file (223663\_He\_HP2\_C2\_m\_18p1GPa\_Rietveld.cif) for the so refined structure are included in the provided supplementary information.

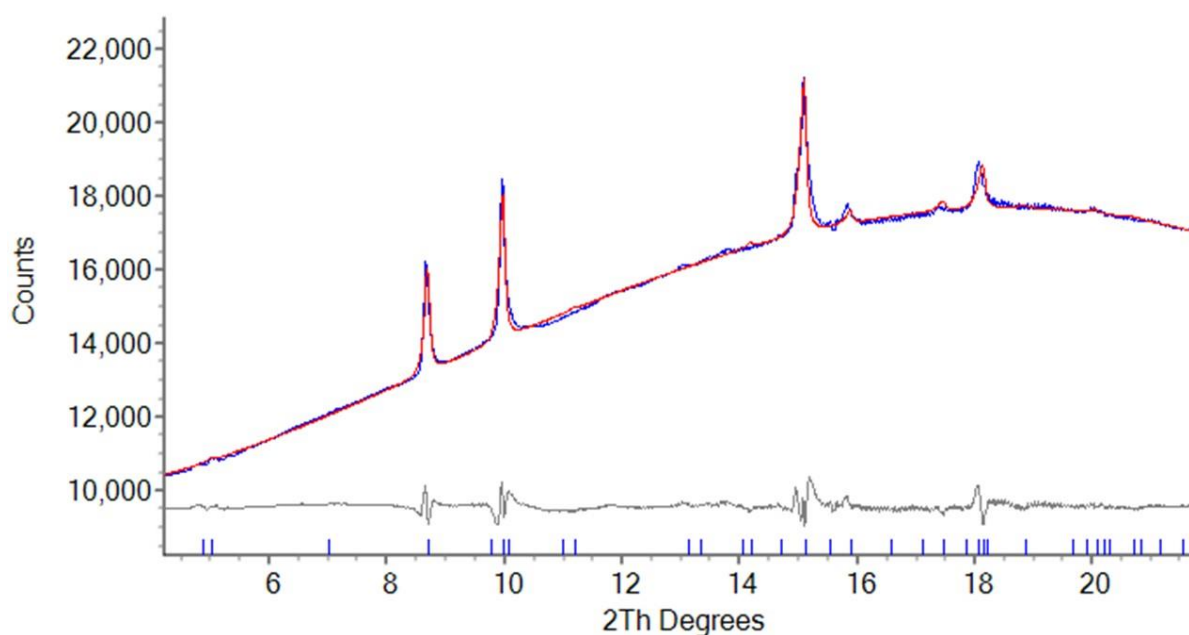

**Figure S6** – Experimental (blue), calculated (red), and difference (grey) patterns for the Rietveld refinement of HP-II (Haines et al.'s model) at 18.5 GPa in He pressure medium. Peak positions are indicated by blue marks.  $R_{wp} = 0.55\%$ ,  $\chi^2 = 0.68$

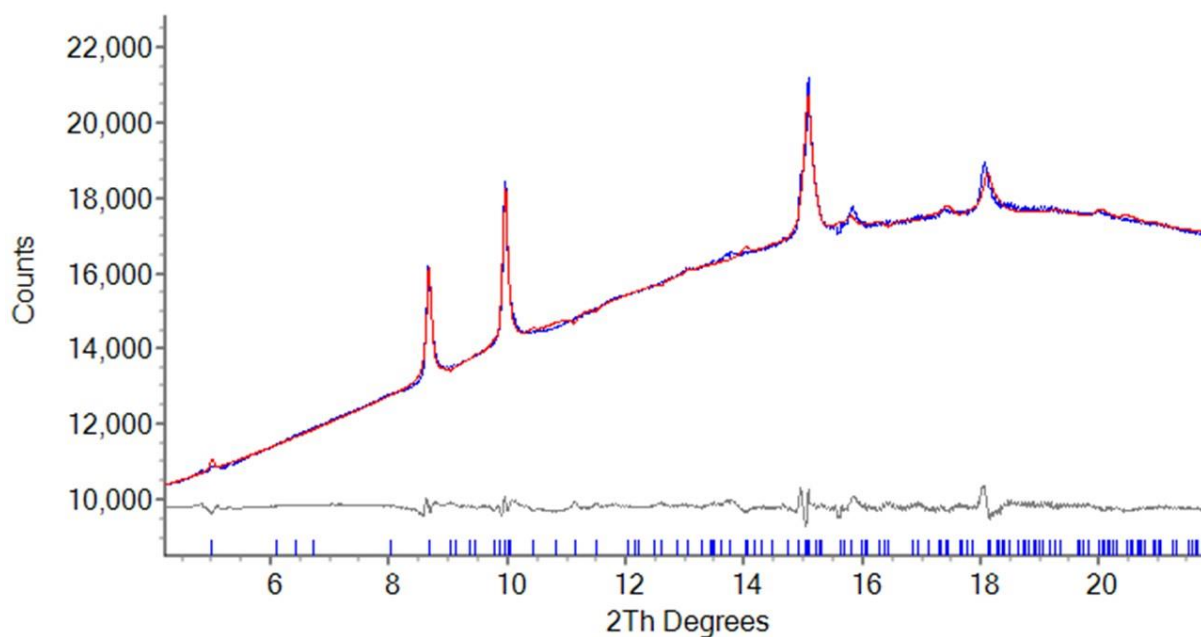

**Figure S7** – Experimental (blue), calculated (red), and difference (grey) patterns for the Rietveld refinement of HP-II (Wang et al.'s model) at 18.5 GPa in He pressure medium. Peak positions are indicated by blue marks.  $R_{wp} = 0.54\%$ ,  $\chi^2 = 0.68$

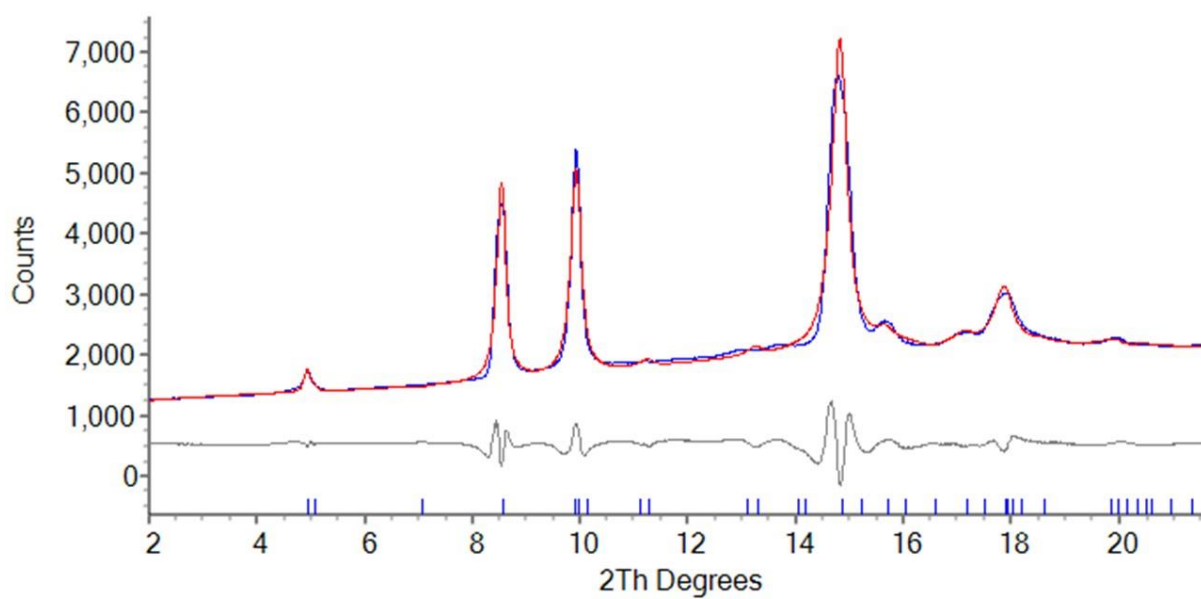

**Figure S8** – Experimental (blue), calculated (red), and difference (grey) patterns for the Rietveld refinement of HP-II (Haines et al.'s model) at 18.1 GPa with no media. Peak positions are indicated by blue marks.  $R_{wp} = 0.55\%$ ,  $\chi^2 = 0.68$

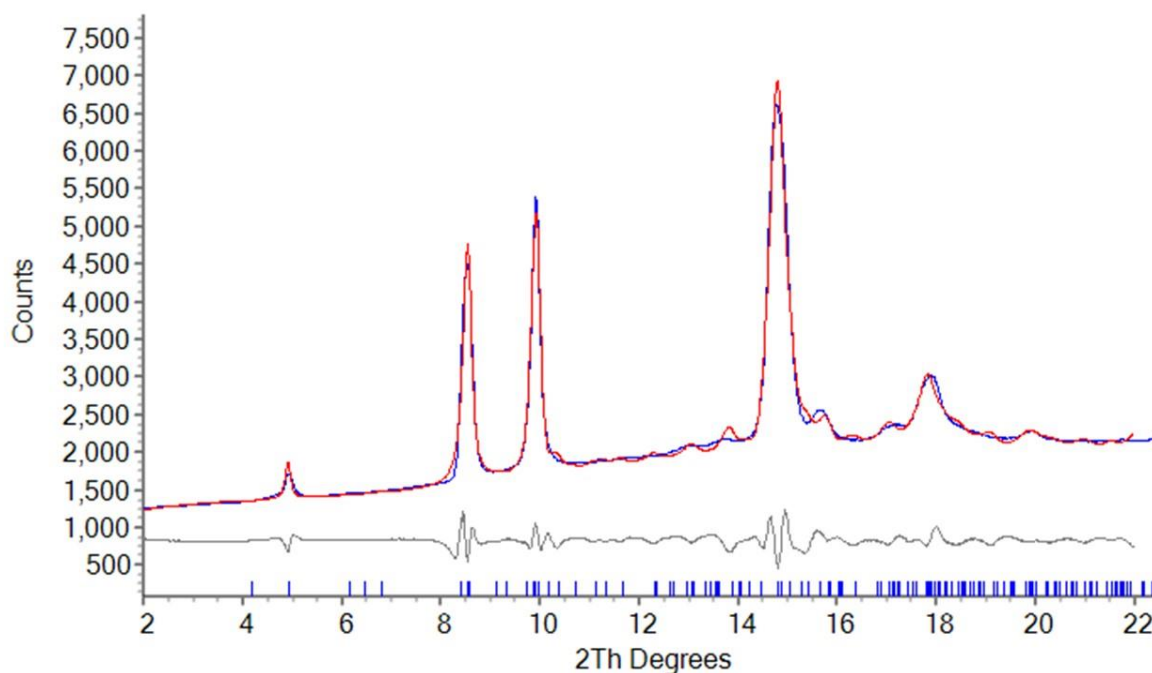

**Figure S9** – Experimental (blue), calculated (red), and difference (grey) patterns for the Rietveld refinement of HP-II (Wang et al.'s model) at 18.1 GPa with no media. Peak positions are indicated by blue marks.  $R_{wp} = 2.63\%$ ,  $\chi^2 = 1.22$

### ***Differences of intra-planar characteristic distance between He medium powder data and other experiments.***

For the comparison of the HP-II unit cell in the high-pressure experiments with helium pressure medium and with no media, a plot of the diffractogram with no media at 18.1 GPa and the background subtracted diffractogram in helium at 18.5 GPa is displayed in Figure S10 for comparison. The difference in peak position for all reflections but (0 0 1) (at  $\sim 5^\circ$ ) is evident, and the large difference in the  $a$  (in-plane) lattice parameter of the trigonal model of HP-II in the two conditions, as noted in the main text and demonstrated by their difference in Figure 3 in the main text, is therefore not a surprise.

### ***Sequential Rietveld refinement of data collected with He medium.***

Sequential Rietveld refinement were used for the cell parameters of HP-II using both models proposed in the literature. A shifted Chebyshev function with 6 parameters was used to fit the background. No structural parameters other than lattice parameters were refined. Minimum and maximum values of  $0.1 \text{ \AA}^2$  and  $1 \text{ \AA}^2$  were set for the thermal parameters (one for each atomic species). Spherical harmonics were used to model preferred orientation. One isotropic Lorentzian parameter was used to model the crystal size contribution to peak. An anisotropic model including Gaussian and Lorentzian terms was used for sample microstrain contribution instead.<sup>8</sup> Table S2 reports structural parameters as obtained from the sequential refinements,  $R_{wp}$  and  $\chi^2$  goodness of fit indices. The input file, integrated data, and cif files of the refined Haines et al.'s model for each pressure are included in the provided supplementary information. The plot in Figure S11 shows how the interplanar distance of HP-II as obtained from powder data for Wang et al.'s model compares with the single crystal data analysis.

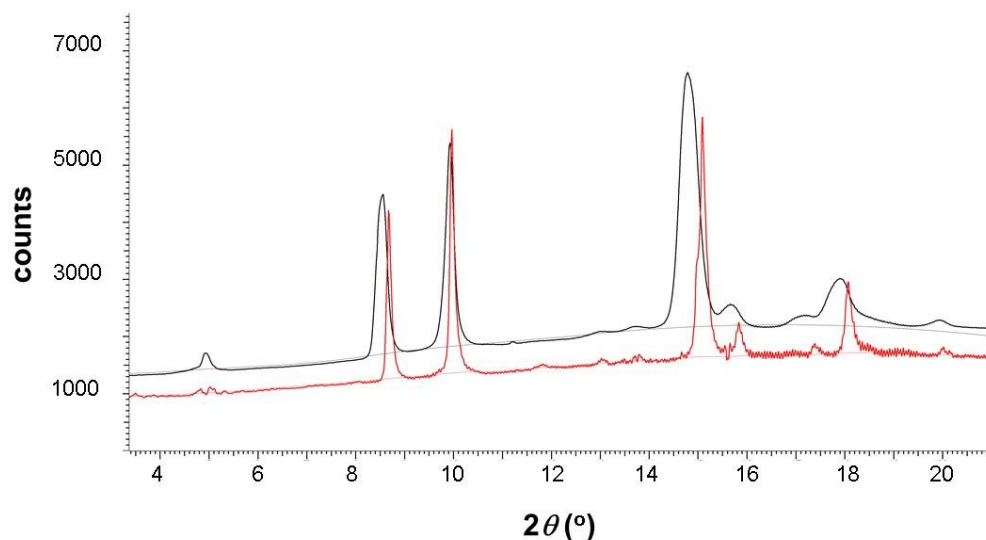

**Figure S10** – Integrated XRD pattern at 18.1 GPa with no media (black line) and background subtracted integrated XRD pattern at 18.5 GPa in He (red line).

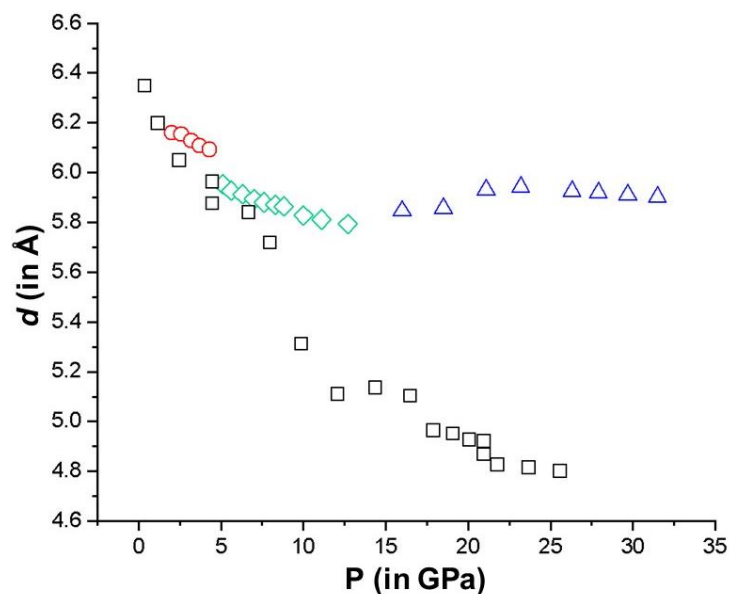

**Figure S11** – A comparison of the interplanar distance  $d(0\ 0\ 1)$  as obtained from single crystal data (black squares) and for Wang's model from powder data in He (blue triangles). HP-0 (red circles) and HP-I (green circles) are shown as obtained from the parametric refinement of powder data in He as described below. The e.s.d. on the values are smaller than the symbols used.

### **Conclusions on the comparison of HP-II structural models**

Wang et al.'s model could not be ruled out on the basis of the chemical soundness or the visual fit and goodness of fit indices which are all very similar in quality to those obtained for Haines et al.'s model. The finding of similar outcomes from refinements of incompatible models is a limitation of Rietveld analysis<sup>9</sup> and single crystal analyses were essential to overcome this dilemma. For the case of the HP-II phase of  $\text{FePS}_3$ , the different unit cells

found by Wang et al. and Haines et al. are unsurprising due to the absence of the (0 0 1) peak in the powder diffraction patterns measured by the former, which is key for the determination of the important inter-layer spacing and thus for the correct identification of the other unit cell parameters.

The determined (0 0 1) distance from single crystal measurement shows that the correct indexation of the powder data for the HP-II phase is the trigonal P-31m model by confirming the occurrence of a reduction of the inter-planar spacing upon the transition to HP-II.

## PRESSURE EVOLUTION OF THE HP-0 AND HP-I PHASES

### *Parametric Rietveld refinements – general comments*

Because of correlation problems between unit cell parameters in the monoclinic phases, the evolution of HP-0 and HP-I were followed by parametric Rietveld refinement.<sup>10</sup> The evolution of the interplanar distance of HP-0 and HP-I can be directly monitored by following the (0 0 1) peak. However, for the powder data with He, there remain very strong correlation problems between the in-plane unit cell parameters, nominally *a* and *b* also with the parametrization and constraints used here. These correlations are much less pronounced in the parametric refinement for the powder data with no media.

### *Parametric Rietveld refinement of data collected with He medium*

Due to insufficient data quality at higher diffraction angle, the parametric refinement had to be performed in the two theta range up to 14 degrees only. The integrated raw datafiles were normalized using a procedure based on the scale factor of the empirical background in a whole pattern refinement.<sup>11</sup> The scale factors *S* of the two phases were constrained to a Boltzmann function:

$$S = \frac{A_1 - A_2}{1 + e^{(x - x_0)/dx}} + A_2 \quad \text{Supplementary Equation 1}$$

Of which parameters *A*<sub>1</sub> is the initial scale factor, *A*<sub>2</sub> the final scale factor, *x*<sub>0</sub> is the pressure at which the scale factor is halfway between *A*<sub>1</sub> and *A*<sub>2</sub>, *dx* affects how steep the sigmoidal function is. *A*<sub>1</sub> (one for each phase), *A*<sub>2</sub> (one for each phase), *x*<sub>0</sub>, *dx* were set as refinable parameters. We report lattice parameters of the most abundant phase only for the HP-0 to HP-I phase transition. The background was modelled using the same empirical background used for the normalization procedure plus a shifted Chebyshev function with 2 parameters. At each pressure step, all lattice parameters were varied so that the two phases were constrained to have the same interplanar distance, *c*\*. One March-Dollase parameter was used for (0 0 1) direction for HP-0, and it was refined to the same value for all scans. Spherical harmonics were used to model preferred orientation for HP-I. One isotropic Lorentzian parameter was used to model the crystal size contribution to peak. An anisotropic model<sup>8</sup> including Gaussian and Lorentzian terms was used for sample microstrain contribution instead. Table S3 reports structural parameters as obtained from the parametric refinements, *R*<sub>wp</sub> and  $\chi^2$  goodness of fit indices. Figures S12 and S13 show some representative Rietveld refinement plot. The input file, integrated data, and output files containing the refined unit cell parameters for each pressure are included in the provided supplementary information.

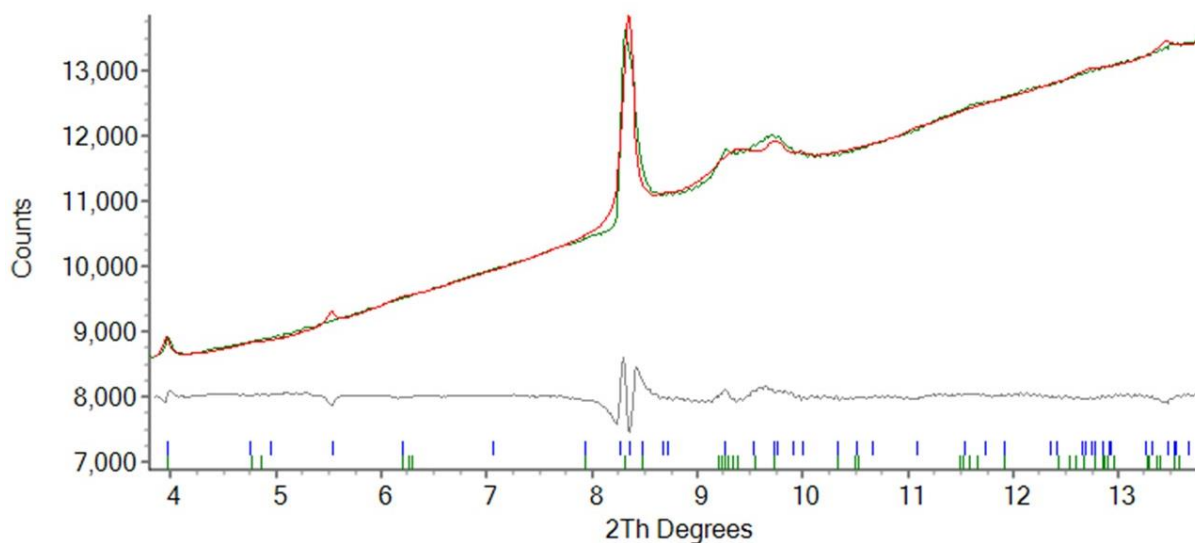

**Figure S12** – Experimental (green), calculated (red), and difference (grey) patterns for the parametric Rietveld refinement of HP-0 and HP-I at 2.6 GPa in He pressure medium. HP-0 and HP-I peak positions are indicated by blue marks and green marks respectively. Refinement parameters are given in Table S3.

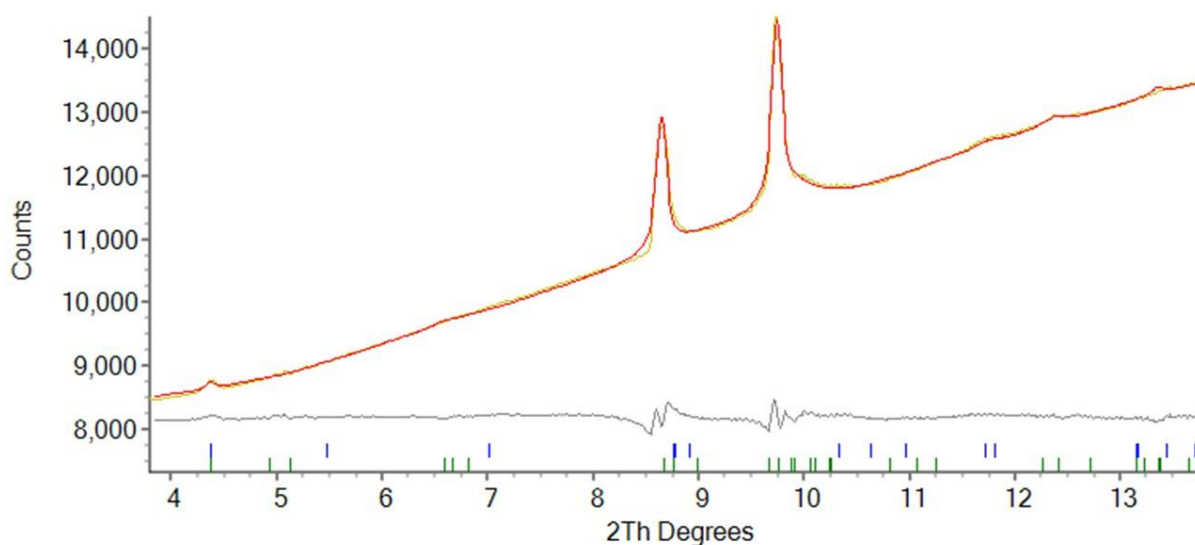

**Figure S13** – Experimental (yellow), calculated (red), and difference (grey) patterns for the parametric Rietveld refinement of HP-0 and HP-I at 12.7 GPa in He pressure medium. HP-0 and HP-I peak positions are indicated by blue marks and green marks respectively. Refinement parameters are given in Table S3.

### ***Parametric Rietveld refinement of data collected without He medium***

The scale factors of the two phases were constrained to a Boltzmann function as in Supplementary Equation 1.  $A_1$  (one for each phase),  $A_2$  (one for each phase),  $x_0$ ,  $dx$  were set as refinable parameters. We report lattice parameters of the most abundant phase only for the HP-0 to HP-I phase transition. The background was modelled using an empirical background obtained from one of the scans plus a shifted Chebyshev function with 5 parameters. At each pressure step, all lattice parameters were varied so that the two

phases were constrained to have the same interplanar distance,  $c^*$ . Spherical harmonics parameters were used to model preferred orientation of HP-0, and they were refined to the same values for all scans. Spherical harmonics parameters were used to also model preferred orientation of HP-I, and they were refined to the same values for all scans up to 7 GPa - they were left to refine independently above that threshold. One isotropic Lorentzian parameter was used to model the crystal size contribution to peak. An anisotropic model<sup>8</sup> including Gaussian and Lorentzian terms was used for sample microstrain contribution instead. Table S4 reports structural parameters as obtained from the parametric refinements,  $R_{wp}$  and  $\chi^2$  goodness of fit indices. Figures S14 to S16 show some representative Rietveld refinement plots. The input file, integrated data, and output files containing the refined unit cell parameters for each pressure are included in the provided supplementary information.

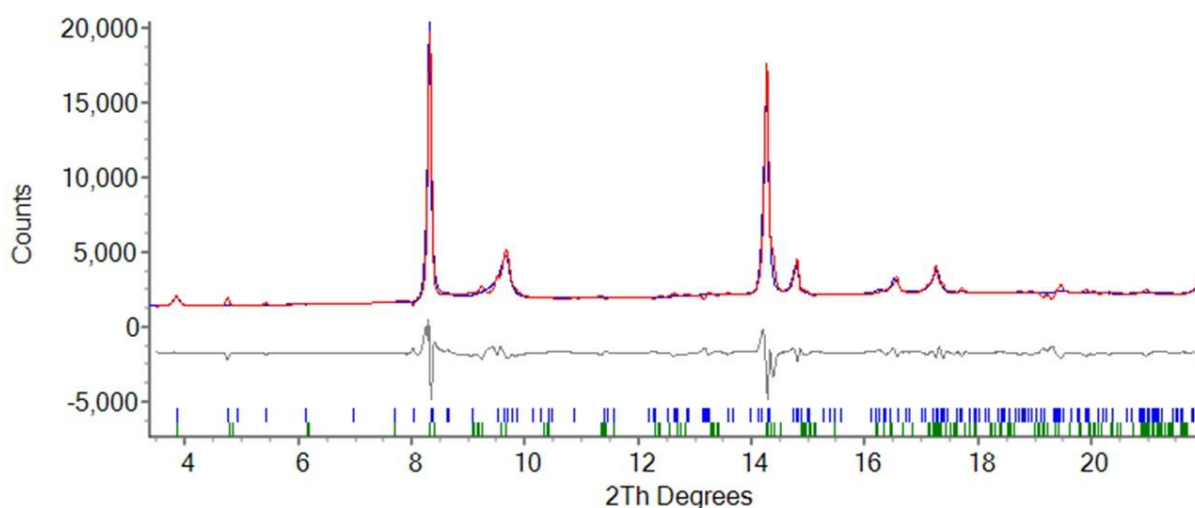

**Figure S14** – Experimental (green), calculated (red), and difference (grey) patterns for the parametric Rietveld refinement of HP-0 and HP-I at 1.1 GPa with no pressure media. HP-0 and HP-I peak positions are indicated by blue marks and green marks respectively. Refinement parameters are given in Table S4.

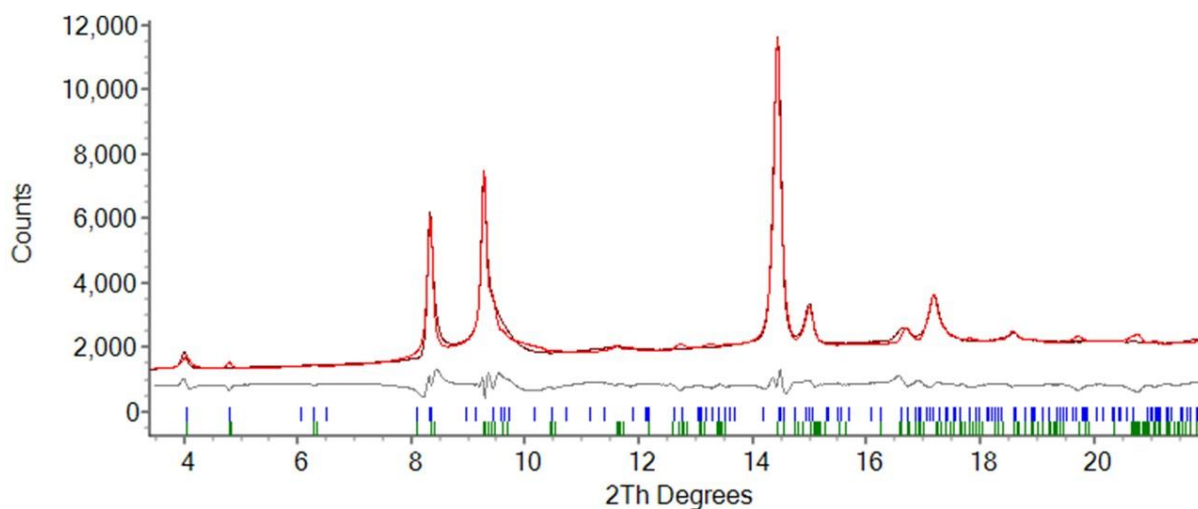

**Figure S15** – Experimental (brown), calculated (red), and difference (grey) patterns for the parametric Rietveld refinement of HP-0 and HP-I at 4.8 GPa with no pressure media. HP-0 and HP-I peak positions are indicated by blue marks and green marks respectively. Refinement parameters are given in Table S4.

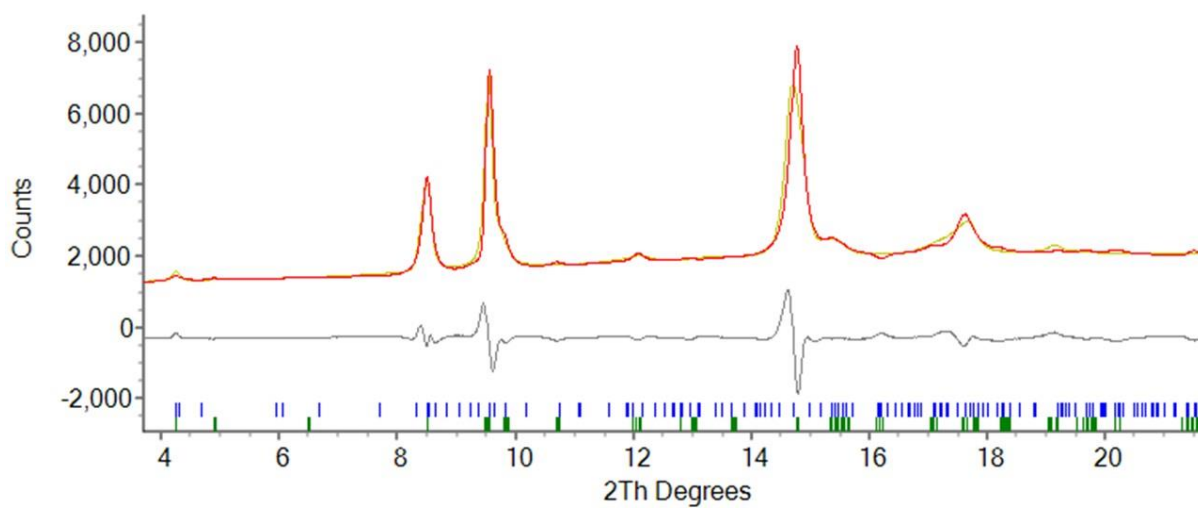

**Figure S16** – Experimental (yellow), calculated (red), and difference (grey) patterns for the parametric Rietveld refinement of HP-0 and HP-I at 12.5 GPa with no pressure media. HP-0 and HP-I peak positions are indicated by blue marks and green marks respectively. Refinement parameters are given in Table S4.

Table S2: output parameters from the sequential Rietveld refinement of the high-pressure powder data with He pressure medium using the two different models for HP-II.

| HP-II (Haines et al.) |      |          |                   |          |                   |                       |          |
|-----------------------|------|----------|-------------------|----------|-------------------|-----------------------|----------|
| file number           | GPa  | <i>a</i> | <i>a</i> (e.s.d.) | <i>c</i> | <i>c</i> (e.s.d.) | <i>R<sub>wp</sub></i> | $\chi^2$ |
| 223611                | 13.9 | 5.613137 | 0.000987          | 5.121194 | 0.00265           | 0.668                 | 0.866    |
| 223612                | 16   | 5.60358  | 0.000989          | 5.060212 | 0.002064          | 0.639                 | 0.819    |
| 223613                | 18.5 | 5.591118 | 0.000891          | 4.976549 | 0.002293          | 0.652                 | 0.81     |
| 223614                | 21.1 | 5.578451 | 0.000961          | 4.912179 | 0.00226           | 0.662                 | 0.83     |
| 223615                | 23.2 | 5.569328 | 0.000925          | 4.861298 | 0.00218           | 0.663                 | 0.834    |
| 223619                | 26.3 | 5.552505 | 0.000853          | 4.807448 | 0.002044          | 0.658                 | 0.854    |
| 223620                | 27.9 | 5.550361 | 0.000913          | 4.773563 | 0.002119          | 0.653                 | 0.81     |
| 223621                | 29.7 | 5.536802 | 0.000874          | 4.746288 | 0.002266          | 0.706                 | 0.927    |
| 223622                | 31.5 | 5.529085 | 0.000869          | 4.714478 | 0.002201          | 0.669                 | 0.876    |

  

| HP-II (Wang et al.) |      |          |                   |          |                   |          |                   |          |                  |                       |          |
|---------------------|------|----------|-------------------|----------|-------------------|----------|-------------------|----------|------------------|-----------------------|----------|
| file number         | GPa  | <i>a</i> | <i>a</i> (e.s.d.) | <i>b</i> | <i>b</i> (e.s.d.) | <i>c</i> | <i>c</i> (e.s.d.) | $\beta$  | $\beta$ (e.s.d.) | <i>R<sub>wp</sub></i> | $\chi^2$ |
| 223611              | 13.9 | 5.65567  | 0.164353          | 9.566439 | 0.278533          | 6.004289 | 0.173879          | 84.90169 | 0.088182         | 0.447                 | 0.556    |
| 223612              | 16   | 5.643483 | 0.067253          | 9.601399 | 0.113992          | 5.865326 | 0.070677          | 85.24682 | 0.027936         | 0.304                 | 0.374    |
| 223613              | 18.5 | 5.634649 | 0.073418          | 9.566651 | 0.124034          | 5.881434 | 0.076344          | 84.69002 | 0.018684         | 0.283                 | 0.338    |
| 223614              | 21.1 | 5.630488 | 0.091008          | 9.55829  | 0.154369          | 5.964352 | 0.095384          | 83.79681 | 0.118631         | 0.303                 | 0.365    |
| 223615              | 23.2 | 5.628582 | 0.062037          | 9.543132 | 0.104293          | 5.982563 | 0.065719          | 83.20275 | 0.0573           | 0.285                 | 0.344    |
| 223619              | 26.3 | 5.617824 | 0.038583          | 9.522352 | 0.064118          | 5.97122  | 0.041303          | 82.86151 | 0.05454          | 0.249                 | 0.31     |
| 223620              | 27.9 | 5.617848 | 0.057742          | 9.526777 | 0.096871          | 5.96687  | 0.061224          | 82.6128  | 0.05758          | 0.244                 | 0.29     |
| 223621              | 29.7 | 5.612299 | 0.081547          | 9.51447  | 0.137005          | 5.961721 | 0.086486          | 82.39197 | 0.050929         | 0.243                 | 0.306    |
| 223622              | 31.5 | 5.606428 | 0.070782          | 9.494225 | 0.119091          | 5.957055 | 0.075199          | 82.1807  | 0.053701         | 0.224                 | 0.282    |

Table S3: output parameters from the parametric Rietveld refinement of the high-pressure powder data with He pressure medium

| HP-0        |      |          |                   |          |                   |          |                   |          |                  |                  |                   |                        |          |
|-------------|------|----------|-------------------|----------|-------------------|----------|-------------------|----------|------------------|------------------|-------------------|------------------------|----------|
| file number | GPa  | <i>a</i> | <i>a</i> (e.s.d.) | <i>b</i> | <i>b</i> (e.s.d.) | <i>c</i> | <i>c</i> (e.s.d.) | $\beta$  | $\beta$ (e.s.d.) | <i>d</i> (0 0 1) | <i>d</i> (e.s.d.) | <i>R</i> <sub>wp</sub> | $\chi^2$ |
| 223557      | 2    | 5.82333  | 0.01563           | 10.22461 | 0.01315           | 6.40742  | 0.00956           | 105.4796 | 0.1903           | 6.174995         | 0.010801          | 0.82                   | 0.88     |
| 223559      | 2.6  | 5.83919  | 0.02094           | 10.22001 | 0.01829           | 6.38371  | 0.01183           | 106.1684 | 0.27701          | 6.131217         | 0.014219          | 0.7                    | 0.76     |
| 223560      | 3.2  | 5.84296  | 0.02576           | 10.22639 | 0.02236           | 6.36328  | 0.01309           | 106.6215 | 0.29191          | 6.097392         | 0.015562          | 0.74                   | 0.81     |
| HP-I        |      |          |                   |          |                   |          |                   |          |                  |                  |                   |                        |          |
| file number | GPa  | <i>a</i> | <i>a</i> (e.s.d.) | <i>b</i> | <i>b</i> (e.s.d.) | <i>c</i> | <i>c</i> (e.s.d.) | $\beta$  | $\beta$ (e.s.d.) | <i>d</i> (0 0 1) | <i>d</i> (e.s.d.) | <i>R</i> <sub>wp</sub> | $\chi^2$ |
| 223561      | 3.7  | 5.65585  | 0.08476           | 10.18894 | 0.05131           | 6.06185  | 0.01025           | 90.21623 | 0.68534          | 6.061807         | 0.010264          | 0.75                   | 0.82     |
| 223562      | 4.3  | 5.59727  | 0.02533           | 10.18234 | 0.04722           | 5.97786  | 0.01059           | 90.20782 | 0.48478          | 5.977821         | 0.010571          | 0.67                   | 0.73     |
| 223566      | 5.1  | 5.5581   | 0.01909           | 10.17734 | 0.03475           | 5.96836  | 0.01157           | 90.33544 | 0.34886          | 5.968258         | 0.011549          | 0.57                   | 0.62     |
| 223567      | 5.6  | 5.53742  | 0.02728           | 10.17223 | 0.02968           | 5.94837  | 0.01351           | 90.49661 | 0.34523          | 5.948147         | 0.013481          | 0.7                    | 0.77     |
| 223570      | 6.3  | 5.53277  | 0.01737           | 10.1504  | 0.0233            | 5.91647  | 0.0124            | 90.60104 | 0.15634          | 5.916144         | 0.012379          | 0.55                   | 0.6      |
| 223571      | 7    | 5.51202  | 0.01998           | 10.14703 | 0.01605           | 5.88348  | 0.01299           | 90.70237 | 0.16085          | 5.883038         | 0.012958          | 0.54                   | 0.59     |
| 223574      | 7.6  | 5.5104   | 0.01971           | 10.11579 | 0.015             | 5.86599  | 0.01529           | 90.76843 | 0.18805          | 5.865462         | 0.015259          | 0.49                   | 0.54     |
| 223575      | 8.3  | 5.50168  | 0.01944           | 10.09575 | 0.01448           | 5.84641  | 0.01974           | 90.87098 | 0.22786          | 5.845735         | 0.019698          | 0.56                   | 0.62     |
| 223576      | 8.8  | 5.49033  | 0.01841           | 10.078   | 0.01383           | 5.82679  | 0.02432           | 90.83062 | 0.15377          | 5.826178         | 0.024268          | 0.52                   | 0.57     |
| 223601      | 10   | 5.45689  | 0.05129           | 10.0523  | 0.03616           | 5.76671  | 0.01566           | 90.83821 | 0.14497          | 5.766093         | 0.015631          | 0.47                   | 0.52     |
| 223606      | 11.1 | 5.47148  | 0.04516           | 10.00419 | 0.03129           | 5.72605  | 0.01445           | 90.82863 | 0.21695          | 5.725451         | 0.014423          | 0.59                   | 0.64     |
| 223607      | 12.7 | 5.41664  | 0.04093           | 9.85601  | 0.02923           | 5.55935  | 0.02105           | 91.3898  | 0.21019          | 5.557715         | 0.021008          | 0.44                   | 0.48     |

Table S4: output parameters from the parametric Rietveld refinement of the high-pressure powder data with no pressure media.

| HP-0        |      |          |                   |          |                   |          |                   |          |                   |                  |                   |                        |          |
|-------------|------|----------|-------------------|----------|-------------------|----------|-------------------|----------|-------------------|------------------|-------------------|------------------------|----------|
| file number | GPa  | <i>a</i> | <i>a</i> (e.s.d.) | <i>b</i> | <i>b</i> (e.s.d.) | <i>c</i> | <i>c</i> (e.s.d.) | $\beta$  | $\beta$ (e.s.d.)  | <i>d</i> (0 0 1) | <i>d</i> (e.s.d.) | <i>R</i> <sub>wp</sub> | $\chi^2$ |
| 223641      | 1.1  | 5.89738  | 0.0006            | 10.23114 | 0.00039           | 106.6814 | 0.02208           | 6.587324 | 0.002889          | 6.31001          | 0.00231           | 7.6                    | 3.69     |
| 223642      | 1.6  | 5.86545  | 0.0008            | 10.21968 | 0.00076           | 105.9033 | 0.03012           | 6.535181 | 0.002643          | 6.28515          | 0.00174           | 4.3                    | 2.09     |
| 223643      | 2.3  | 5.87044  | 0.00231           | 10.21002 | 0.00172           | 105.8725 | 0.07001           | 6.522465 | 0.005351          | 6.27287          | 0.00296           | 5.48                   | 2.65     |
| 223646      | 2.7  | 5.8452   | 0.00234           | 10.20395 | 0.00134           | 105.5232 | 0.07165           | 6.441462 | 0.004215          | 6.22855          | 0.00296           | 5.84                   | 2.85     |
| 223648      | 3.3  | 5.85283  | 0.00299           | 10.17935 | 0.00334           | 102.8171 | 0.08814           | 6.404081 | 0.006131          | 6.24161          | 0.00386           | 5.84                   | 2.76     |
| 223649      | 3.6  | 5.82255  | 0.00268           | 10.16452 | 0.00212           | 100.0543 | 0.09435           | 6.328509 | 0.005696          | 6.22729          | 0.0032            | 6.53                   | 3.12     |
| 223650      | 4.1  | 5.7332   | 0.0025            | 10.14381 | 0.00165           | 94.46608 | 0.09696           | 6.199293 | 0.004727          | 6.1758           | 0.00339           | 5.92                   | 2.83     |
| HP-I        |      |          |                   |          |                   |          |                   |          |                   |                  |                   |                        |          |
| file number | GPa  | <i>a</i> | <i>a</i> (e.s.d.) | <i>b</i> | <i>b</i> (e.s.d.) | $\beta$  | $\beta$ (e.s.d.)  | <i>c</i> | <i>c</i> (e.s.d.) | <i>d</i> (0 0 1) | <i>d</i> (e.s.d.) | <i>R</i> <sub>wp</sub> | $\chi^2$ |
| 223651      | 4.8  | 5.78988  | 0.0048            | 10.12559 | 0.00171           | 90.51537 | 0.03605           | 6.007033 | 0.005509          | 6.00528          | 0.00404           | 4.04                   | 1.93     |
| 223652      | 6.5  | 5.79637  | 0.00201           | 10.06309 | 0.00095           | 90.324   | 0.02963           | 5.930885 | 0.004256          | 5.93062          | 0.00342           | 3.97                   | 1.81     |
| 223653      | 7.3  | 5.78289  | 0.00202           | 10.03661 | 0.00093           | 90.33068 | 0.03091           | 5.905848 | 0.004761          | 5.90551          | 0.00403           | 5.59                   | 2.56     |
| 223654      | 9.1  | 5.76586  | 0.00256           | 9.98435  | 0.00119           | 90.23657 | 0.0455            | 5.800089 | 0.006047          | 5.80036          | 0.00491           | 6.05                   | 2.84     |
| 223655      | 10.1 | 5.75548  | 0.00181           | 9.96246  | 0.0018            | 90.15874 | 0.03641           | 5.760842 | 0.00341           | 5.76082          | 0.0028            | 6.07                   | 2.87     |
| 223656      | 11   | 5.74077  | 0.00144           | 9.94451  | 0.00154           | 90.20552 | 0.03435           | 5.743457 | 0.002443          | 5.74351          | 0.00212           | 6.11                   | 2.84     |
| 223657      | 11.8 | 5.73278  | 0.00294           | 9.91681  | 0.00151           | 89.47031 | 0.08829           | 5.732755 | 0.005468          | 5.73188          | 0.00491           | 7.43                   | 3.46     |
| 223658      | 12.5 | 5.71993  | 0.00344           | 9.8907   | 0.00173           | 89.45912 | 0.09813           | 5.712195 | 0.00545           | 5.71155          | 0.00478           | 6.05                   | 2.78     |

## REFERENCES

1. Haines, C. R. S. *et al.* Pressure-Induced Electronic and Structural Phase Evolution in the van der Waals Compound FePS<sub>3</sub>. *PHYSICAL REVIEW LETTERS* **121**, (2018).
2. Wang, Y. *et al.* Emergent superconductivity in an iron-based honeycomb lattice initiated by pressure-driven spin-crossover. *Nature communications* **9**, 1–7 (2018).
3. *CrysAlis PRO*. (Agilent Technologies Ltd, 2014).
4. Murayama, C. *et al.* Crystallographic features related to a van der Waals coupling in the layered chalcogenide FePS<sub>3</sub>. *Journal of Applied Physics* **120**, 142114 (2016).
5. Coelho, A. A. TOPAS and TOPAS-Academic: an optimization program integrating computer algebra and crystallographic objects written in C++. *Journal of Applied Crystallography* **51**, 210–218 (2018).
6. Madsen, I. C. & Scarlett, N. V. Y. Quantitative Phase Analysis. in *Powder Diffraction – Theory and Practice* (eds. Dinnabier, R. E. & Billinge, S. J. L.) (RCS publishing, 2008).
7. Coelho, A. A. *TOPAS-Academic Version 6 - Technical Reference*. (2016).
8. Stephens, P. W. Phenomenological model of anisotropic peak broadening in powder diffraction. *Journal of Applied Crystallography* **32**, 281–289 (1999).
9. Buchsbaum, C. & Schmidt, M. U. Rietveld refinement of a wrong crystal structure. *Acta Crystallographica Section B: Structural Science* **63**, 926–932 (2007).
10. Stinton, G. W. & Evans, J. S. O. Parametric Rietveld refinement. *Journal of Applied Crystallography* **40**, 87–95 (2007).
11. Lampronti, G. I. *et al.* Changing the game of time resolved X-ray diffraction on the mechanochemistry playground by downsizing. *Nature Communications* **12**, 1–9 (2021).
